# Supplementary material for: Interpolating Video-LLMs: Toward Longer-sequence LMMs in a Training-free Manner
Source: arXiv:2409.12963 source file (2024-10-02)
Supplement: Supplementary file 1 [file 7supplemental.tex]

\section{Supplemental Materials}
\subsection{Computational Cost Analysis}
\begin{wraptable}{r}{0.4\linewidth}
  \centering
  \vspace{-0.4in}
  \captionsetup{font=small}
        \caption{FLOPS and BOPS for ResNet-18.}
        \scalebox{0.750}{
        \begin{tabular}{ccc}\toprule
        Method         & BOPS                         & FLOPS                       \\\hline
        BNN  & $1.695\times{10}^9$          & $1.314\times{10}^8$         \\
        XNOR-Net  & $1.695\times{10}^9$          & $1.333\times{10}^8$         \\
        ProxyBNN  & $1.695\times{10}^9$          & $1.564\times{10}^8$         \\
        IR-Net   & $1.676\times{10}^9$          & $1.544\times{10}^8$         \\
        RBNN    & $1.785\times{10}^9$          & $1.644\times{10}^8$         \\
        CMIM           & $1.676\times{10}^9$          & $1.544\times{10}^8$         \\\hline
        Full Precision & $0$                          & $1.826\times{10}^8$         \\\bottomrule
        \end{tabular}}
        \label{tabel:cost}
\end{wraptable}
In Table~\ref{tabel:cost}, we separate the number of binary operations and floating point operations, including all types of operations such as skip structure, max pooling, \textit{etc}. It shows that our method leaves the number of BOPs and the number of FLOPs constant in the model inference stage, even though our method is more computational expensive in the training stage.
